# Supplementary material for: R4: Retrieval-Augmented Reasoning for Vision-Language Models in 4D Spatio-Temporal Space
Source: arXiv:2512.15940 source file (2025-12-17)
Supplement: Supplementary file 1 [file X_suppl.tex]

\clearpage
\setcounter{page}{1}
\maketitlesupplementary

\input{01_Chapter/B_metrics}

Prompts für die Modelle

VQA Prompts: \ref{tab:perspective_prompt}

Context Prompts for LGM:

\begin{table}[t!]
    \centering
    \small
    \begin{tcolorbox}[colframe=black, colback=gray!10, boxrule=0.25mm, width=\linewidth]
        \textbf{Context and Formatting Prompt:} \\
        You are a helpful assistant for navigating an autonomous car based on sensor input and driver instructions. Don't collide, keep safe distance to other vehicles, and decrease speed or brake if necessary. Answer only exactly in this format: \{\textcolor{blue}{\texttt{"steer":}} steer control ranging from \textcolor{blue}{\texttt{-1}} (left) to \textcolor{blue}{\texttt{1}} (right), \textcolor{blue}{\texttt{"throttle":}} acceleration ranging from \textcolor{blue}{\texttt{0}} to \textcolor{blue}{\texttt{1}}, \textcolor{blue}{\texttt{"brake":}} braking ranging from \textcolor{blue}{\texttt{0}} (no brake) to \textcolor{blue}{\texttt{1}} (full brake), \textcolor{blue}{\texttt{"reverse":}} flag for switching between driving \textcolor{blue}{\texttt{forward}} (False) and \textcolor{blue}{\texttt{backward}} (True)\}
    \end{tcolorbox}
    \begin{tcolorbox}[colframe=black, colback=gray!10, boxrule=0.25mm, width=\linewidth]
        \textbf{Camera View Indexing Prompt:} \\
        This is the \textcolor{blue}{\texttt{$<$camera$>$}} cam image: \textcolor{orange}{\texttt{image}} \\
        \textcolor{blue}{\texttt{$<$camera$>$}} $=$ \{ \textcolor{blue}{\texttt{front}} , \textcolor{blue}{\texttt{back}} , \textcolor{blue}{\texttt{left}} , \textcolor{blue}{\texttt{right}} \}
    \end{tcolorbox}
    \caption{\textbf{High-level baseline prompts} for giving minimal context to the model under test for language-guided motion.}
    \label{tab:prompts}
\end{table}

\section{Rationale}
\label{sec:rationale}
Having the supplementary compiled together with the main paper means that:
\begin{itemize}
\item The supplementary can back-reference sections of the main paper, for example, we can refer to \cref{sec:intro};
\item The main paper can forward reference sub-sections within the supplementary explicitly (e.g. referring to a particular experiment); 
\item When submitted to arXiv, the supplementary will already included at the end of the paper.
\end{itemize}
To split the supplementary pages from the main paper, you can use \href{https://support.apple.com/en-ca/guide/preview/prvw11793/mac#:~:text=Delete%20a%20page%20from%20a,or%20choose%20Edit%20%3E%20Delete).}{Preview (on macOS)}, \href{https://www.adobe.com/acrobat/how-to/delete-pages-from-pdf.html#:~:text=Choose%20%E2%80%9CTools%E2%80%9D%20%3E%20%E2%80%9COrganize,or%20pages%20from%20the%20file.}{Adobe Acrobat} (on all OSs), as well as \href{https://superuser.com/questions/517986/is-it-possible-to-delete-some-pages-of-a-pdf-document}{command line tools}.
